# Supplementary material for: Manthan: A Data Driven Approach for Boolean Function Synthesis
Source: arXiv:2005.06922 source file (2020-05-14)
Supplement: Supplementary file 1 [file appendix.tex]

\pagebreak
\section{Cactus plots to show impact of {\phasetwo} and sampling scheme}
\begin{figure}[h]
	\centering
	\includegraphics[scale=0.45]{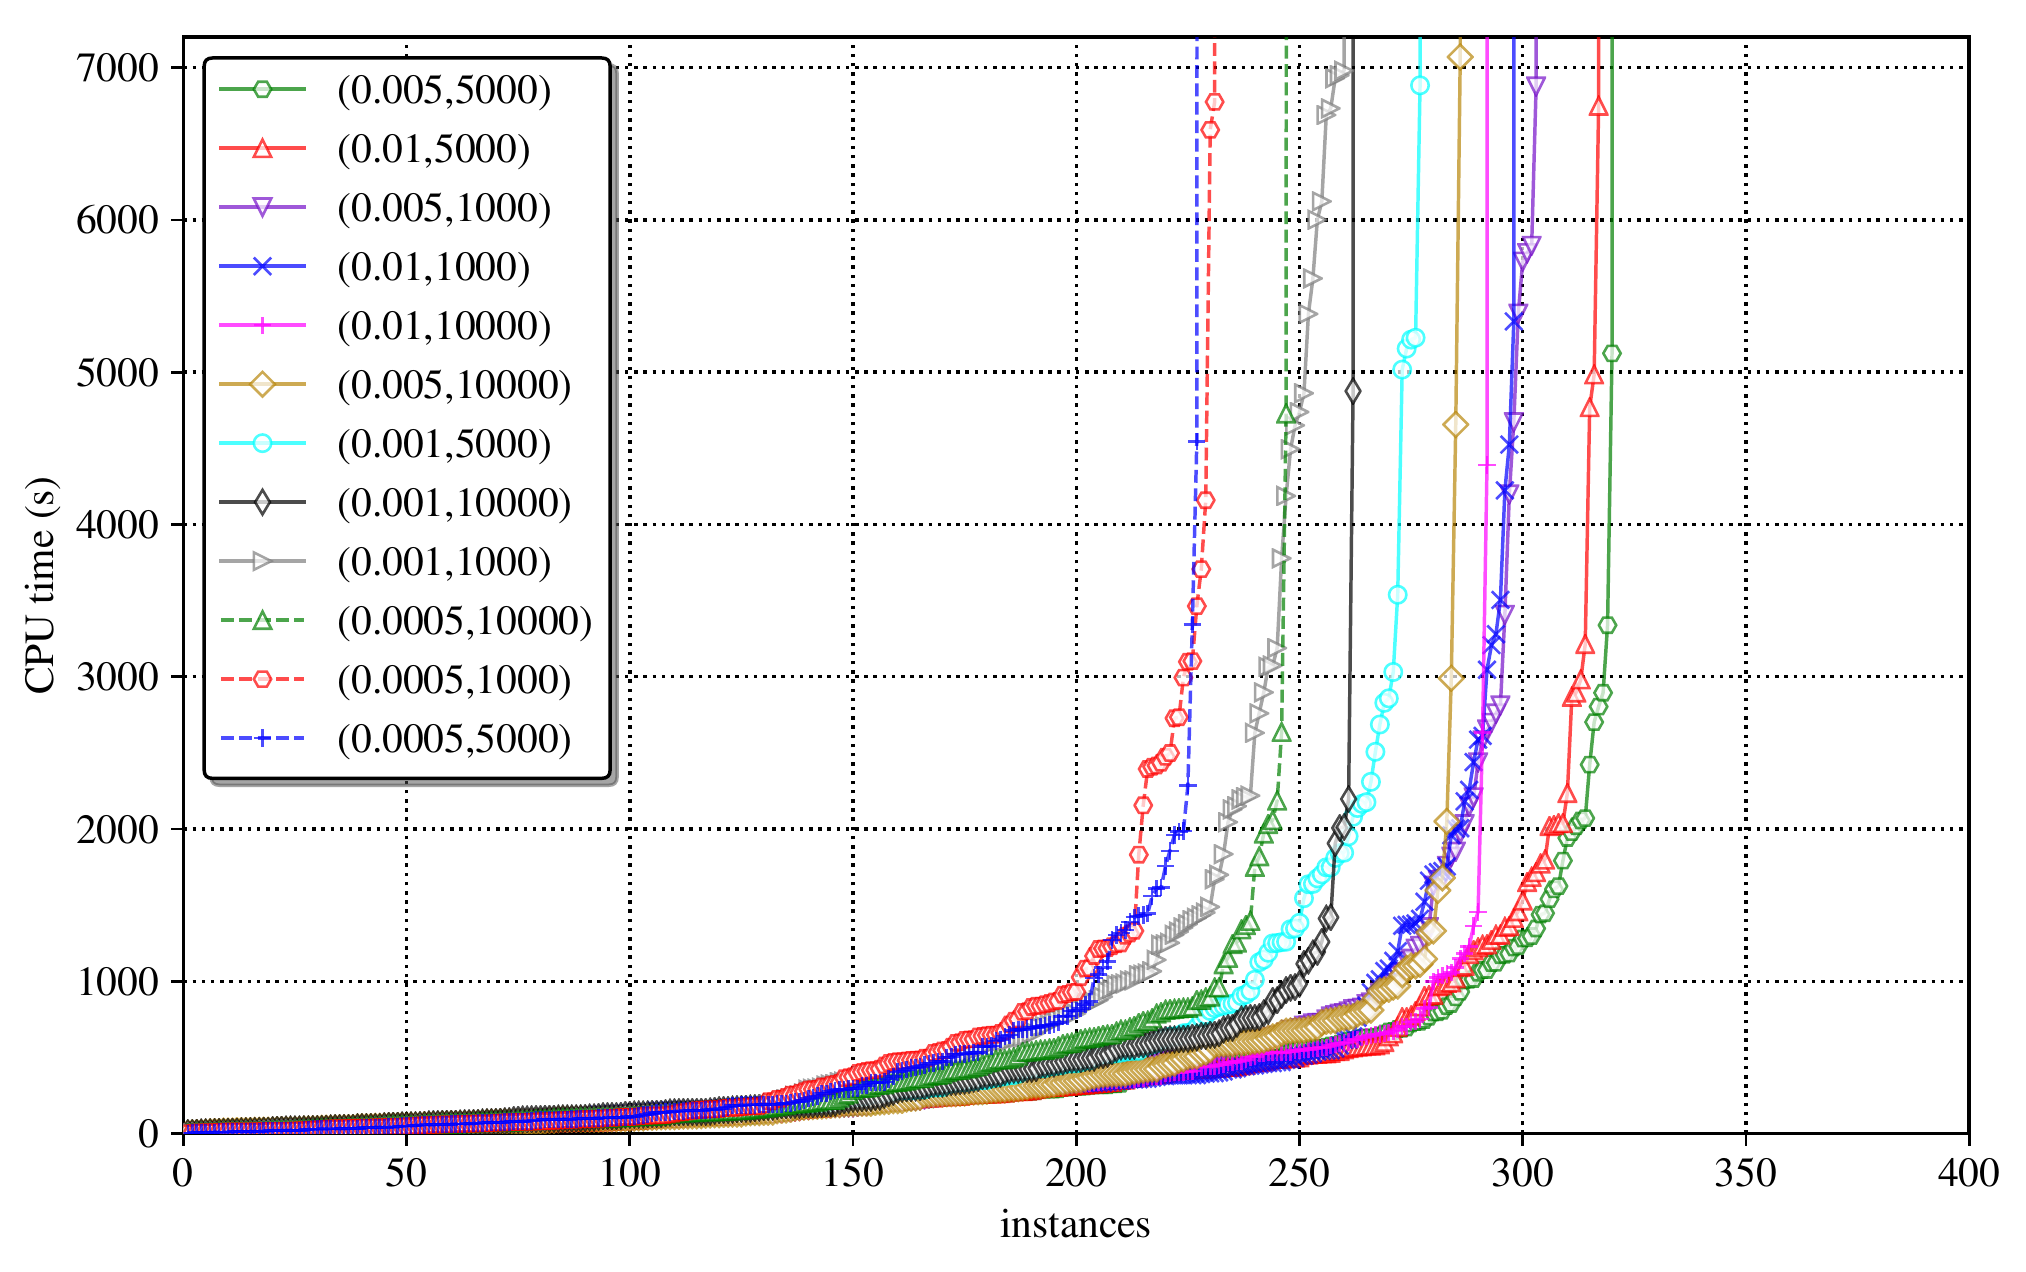}
	\caption{Cactus plot to show performance of {\tool} with different minimum-impurity-decrease and number of samples}
\end{figure}
\begin{figure}[h]
	\centering
	\includegraphics[scale=0.45]{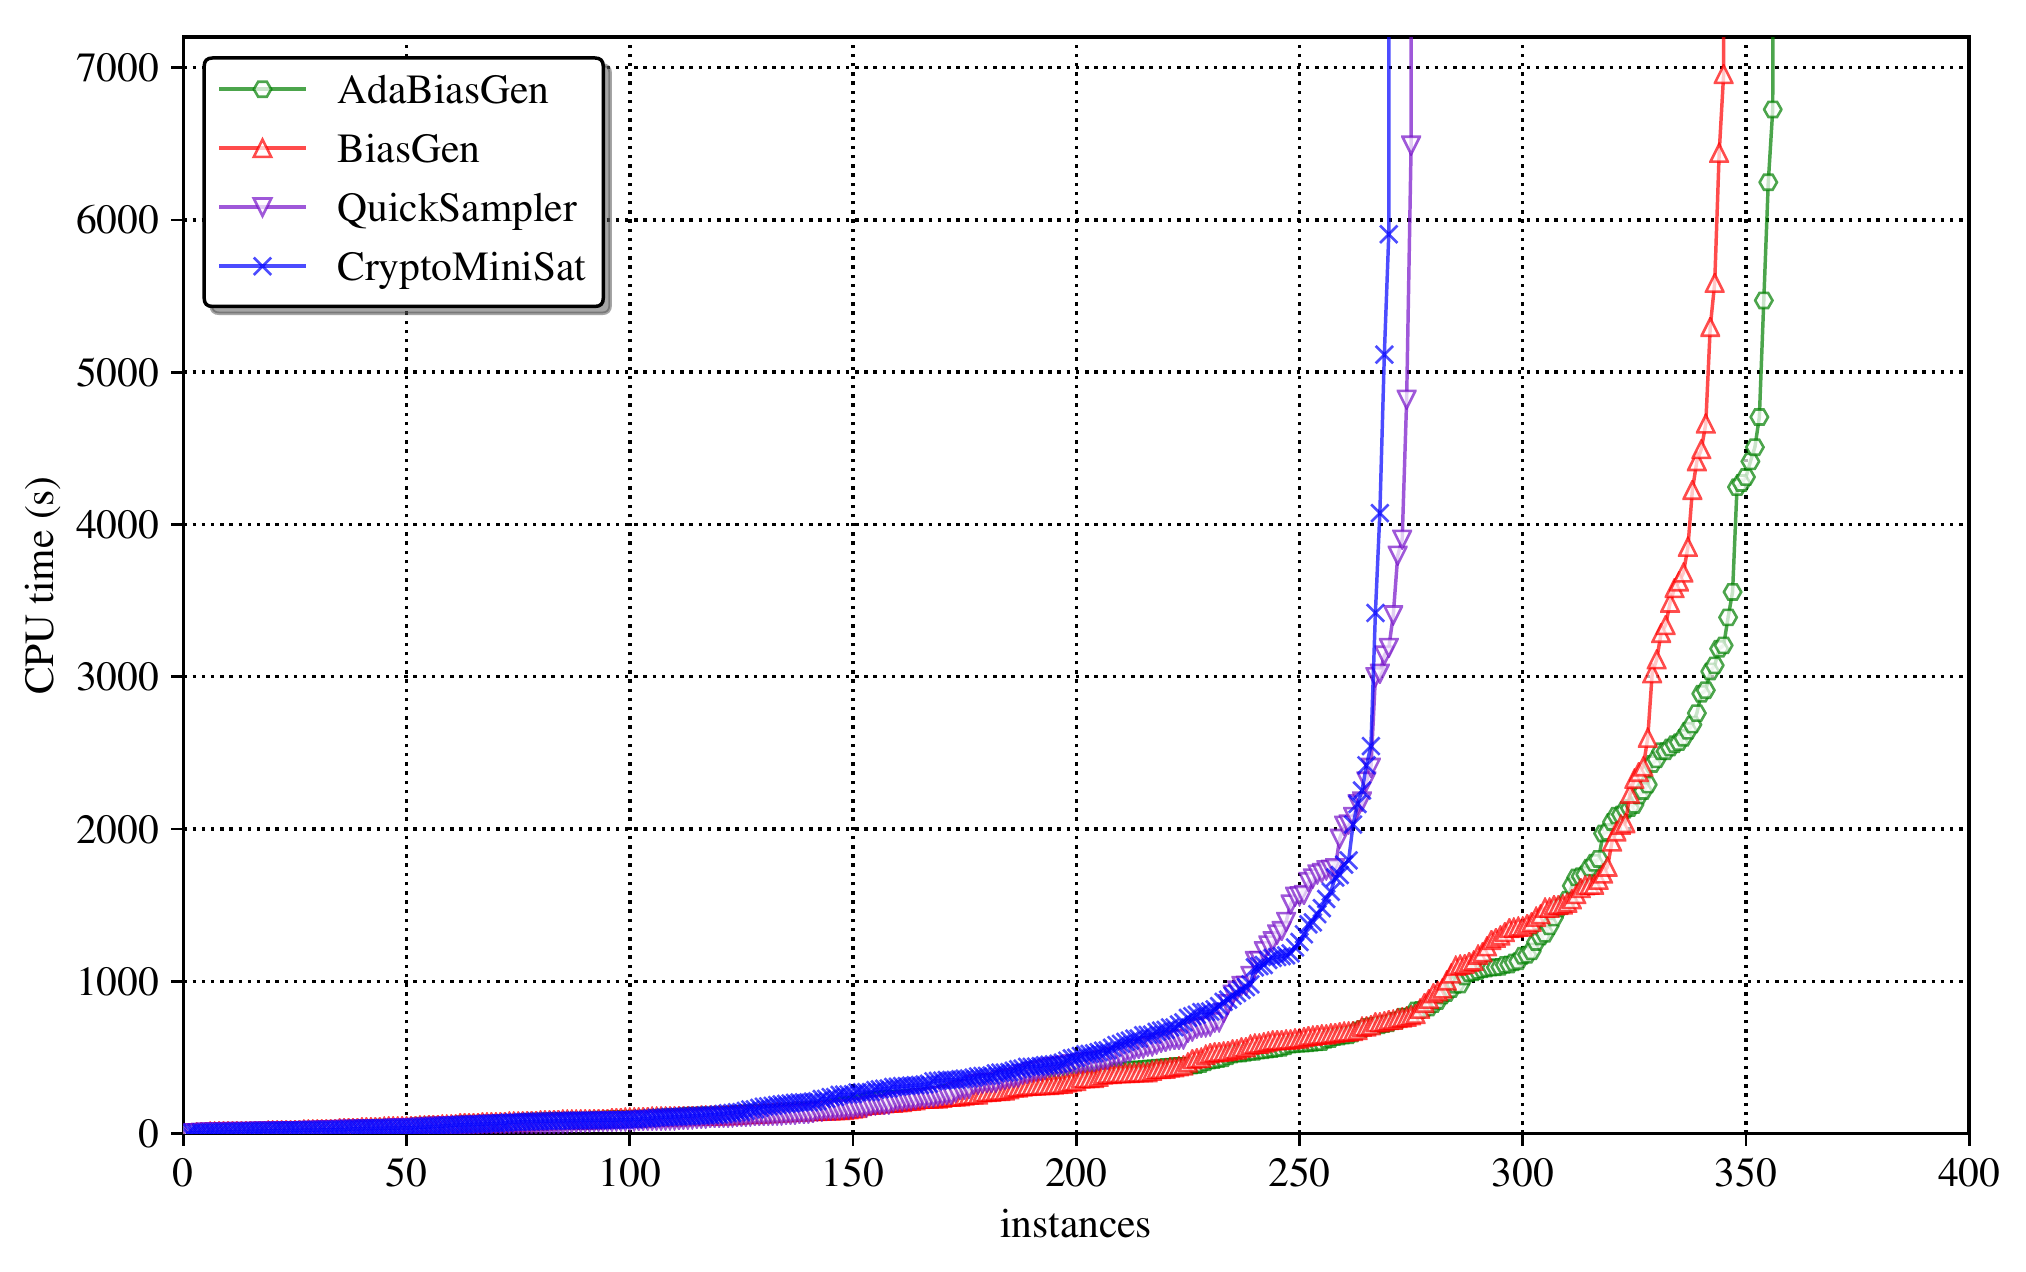}
	\caption{Cactus plot to show performance of {\tool} with different sampling tools}
\end{figure}
